# Supplementary material for: Iniva: Inclusive and Incentive-compatible Vote Aggregation
Source: arXiv:2404.04948 source file (2024-04-07)
Supplement: Supplementary file 1 [file appendix.tex]

\section{Additional Simulations}

In this section, we present the results of some additional simulations conducted. 

\subsection{Gosig Analysis under Large $m$}

In this simulation, we simulate the vote omission attack on Gosig under large values of $m$. 
Figure~\ref{fig:attacker_m} illustrates the results of the simulation. 
Results show that the attack probability in Gosig under large values of $m$ is similar to a star protocol with round robin leader election, which means Gosig inclusiveness for collateral of $0$ is reduced down to $m$.

\begin{figure}[!ht]
\includegraphics[width=\linewidth]{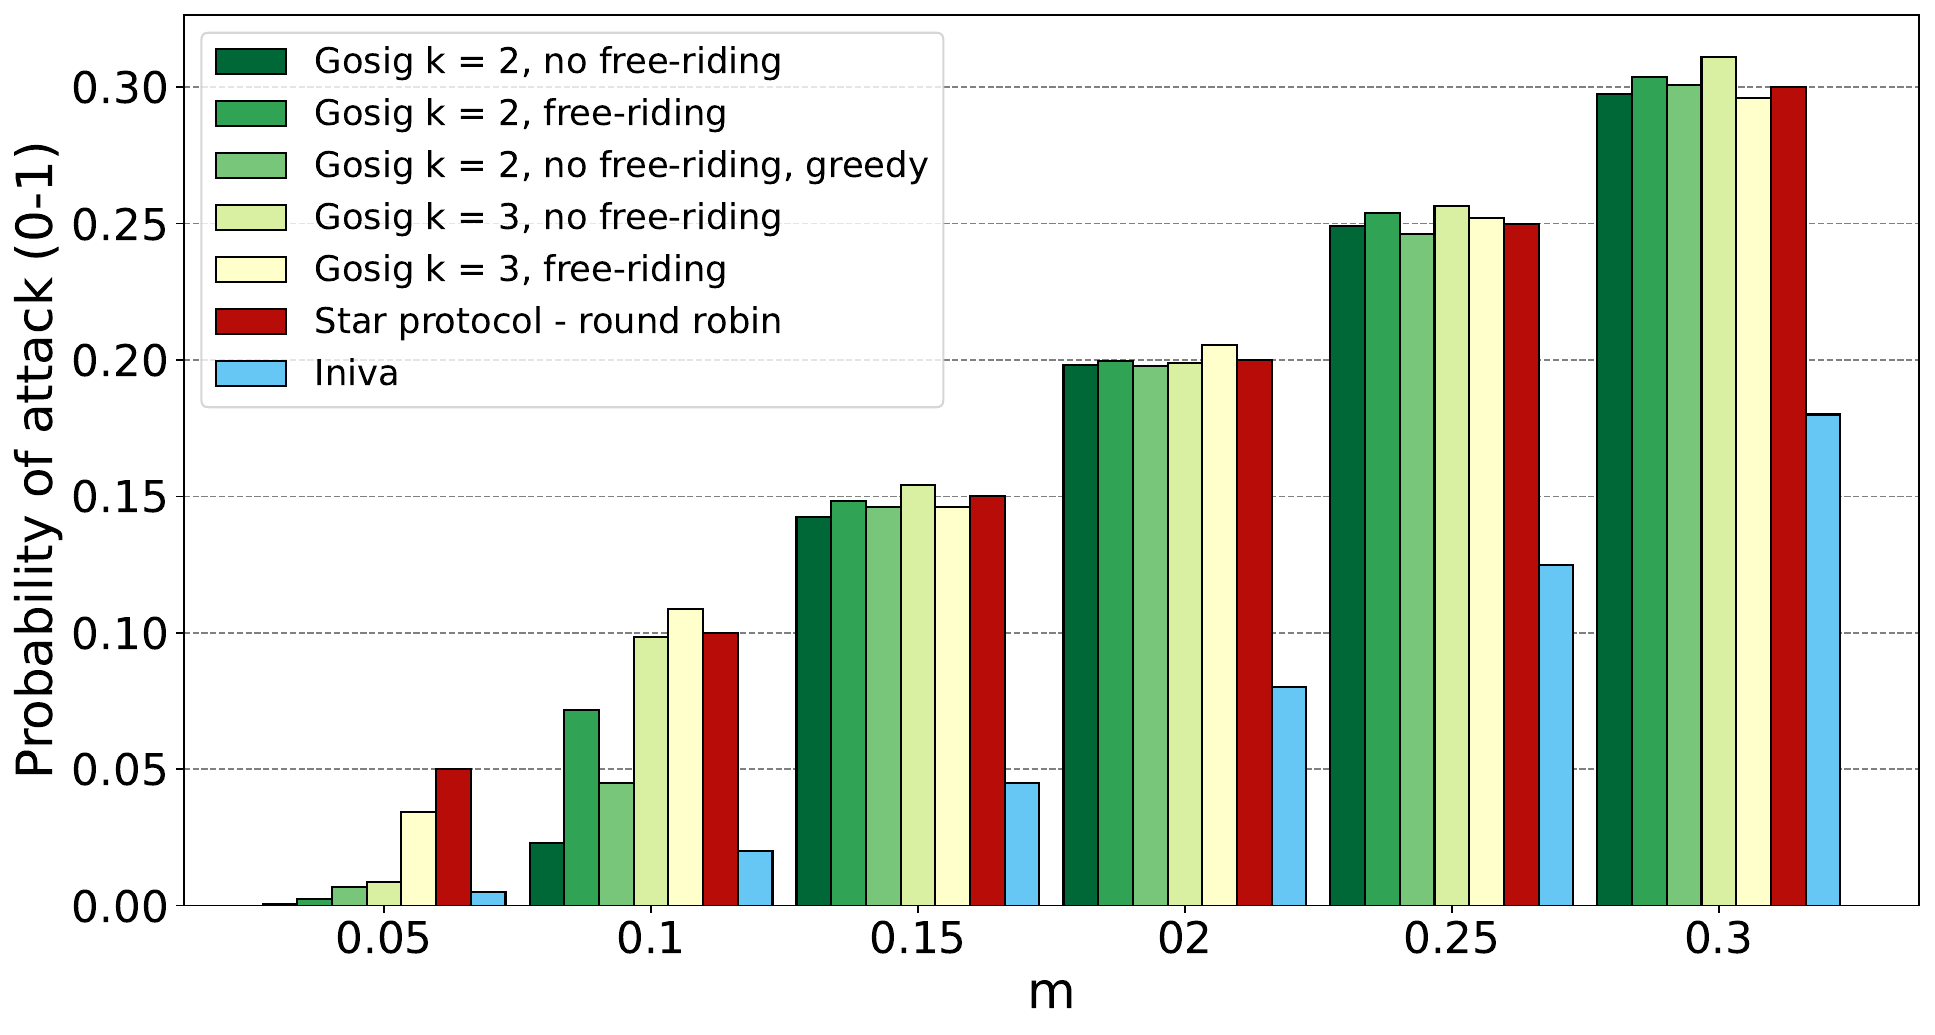}
\caption{This simulation compares the possibility of targeted vote omission attack in Gosig with Star protocol and Iniva under large values of $m$. }
\label{fig:attacker_m}
\end{figure}

\pagebreak
\subsection{Collateral Analysis}

In this simulation, we analyze the security of \proj against vote omission attack under different collateral and attacking power $m$. 
The results are shown in Figure~\ref{fig:collateral_m}.
\proj preserves the $(2 m^2)$-$c$-inclusiveness until collateral of size 5. 
However, as the size of collateral increases, \proj loses the protection against the attack. 
With the collateral of 10 (tree fan-out), \proj becomes $(m)$-$c$-inclusive, since the attacker is able to exclude the victim by removing a whole branch whenever it is the leader. 
Thus, these large attacks are addressed with incentive or reputation-based schemes. 

\begin{figure}[h]
\includegraphics[width=\linewidth]{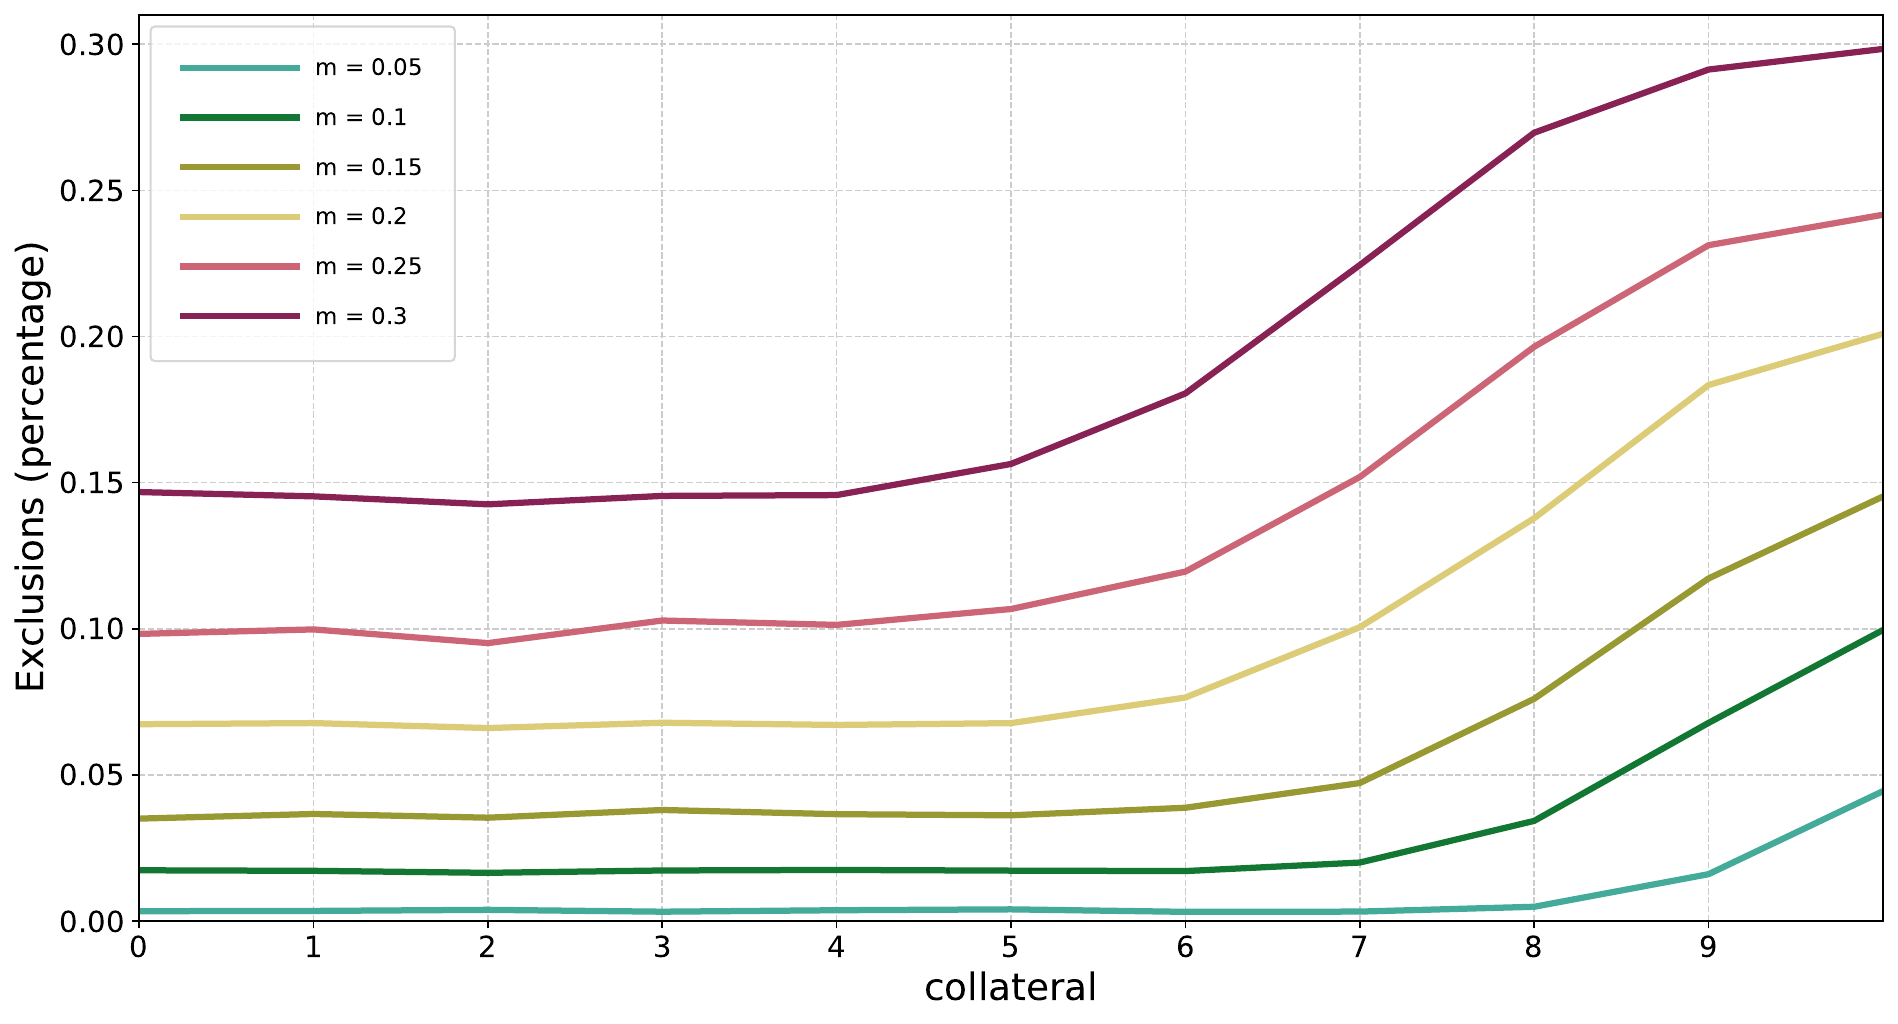}
\caption{The results of the collateral analysis of \proj under different $m$. There are 111 processes in each committee (a full 2-level tree with fan-out = 10). }
\label{fig:collateral_m}
\end{figure}

\section{Additional Experiments}

In the Scaling evaluation, we also measured latency observed for various configurations with and without payload for HotStuff and \proj (shown in Figure~\ref{fig:configlth}).
We observed that the latency is higher in the \proj protocol due to the tree communication model instead of the star communication model of HotStuff.

\begin{figure}[h]
    \centering
        \resizebox{\linewidth}{!}{%
        \input{plots/config_lt.tex}
        }
       \caption{Latency evaluation with batchsize B=100 and 
varying configuration sizes and payloads.
Configuration sizes are selected to have an almost complete tree of height 3.}
\label{fig:configlt}
\end{figure}

\vfill
